# Supplementary material for: CrypTen: Secure Multi-Party Computation Meets Machine Learning
Source: arXiv:2109.00984 source file (2022-09-15)
Supplement: Supplementary file 1 [file appendix.tex]

\documentclass{article}

% if you need to pass options to natbib, use, e.g.:
     \PassOptionsToPackage{numbers, compress}{natbib}
% before loading neurips_2021

% ready for submission
\usepackage{neurips_2021}
 
% to compile a preprint version, e.g., for submission to arXiv, add add the
% [preprint] option:
    % \usepackage[preprint]{neurips_2021}

% to compile a camera-ready version, add the [final] option, e.g.:
%     \usepackage[final]{neurips_2021}

% to avoid loading the natbib package, add option nonatbib:
%    \usepackage[nonatbib]{neurips_2021}

\usepackage[ruled,vlined]{algorithm2e}
\usepackage{algorithmic}
\usepackage[utf8]{inputenc} % allow utf-8 input
\usepackage[T1]{fontenc}    % use 8-bit T1 fonts
\usepackage{hyperref}       % hyperlinks
\usepackage{url}            % simple URL typesetting
\usepackage{booktabs}       % professional-quality tables
\usepackage{amsfonts}       % blackboard math symbols
\usepackage{nicefrac}       % compact symbols for 1/2, etc.
\usepackage{microtype}      % microtypography
\usepackage[table]{xcolor}          % colors
\usepackage{amsmath}
\usepackage{enumitem}
\usepackage{amsthm}
\usepackage{graphicx}
\usepackage{subcaption}
\usepackage{color, colortbl}
\usepackage{wrapfig}
\usepackage{makecell}
\usepackage{listings}
\usepackage{wrapfig}
\usepackage{nicefrac}
\usepackage{multirow}

\newcommand{\crypten}{\textsc{CrypTen}}

\DeclareFixedFont{\ttb}{T1}{txtt}{bx}{n}{7} % for bold
\DeclareFixedFont{\ttm}{T1}{txtt}{m}{n}{7}  % for normal
\DeclareFixedFont{\ttmlarge}{T1}{txtt}{m}{n}{9}  % for normal
\definecolor{deepblue}{rgb}{0,0,0.5}
\definecolor{deepred}{rgb}{0.6,0,0}
\definecolor{deepgreen}{rgb}{0,0.5,0}

\newcommand\pythonstyle{\lstset{
language=Python,
basicstyle=\linespread{0.8}\selectfont\ttm,
commentstyle=\linespread{0.8}\selectfont\ttm\color{deepgreen},
otherkeywords={self},             % Add keywords here
keywordstyle=\linespread{0.8}\selectfont\ttb\color{deepblue},
emph={incmatrix},          % Custom highlighting
emphstyle=\ttb\color{deepred},    % Custom highlighting style
stringstyle=\color{deepgreen},
frame=tb,                         % Any extra options here
showstringspaces=false            % 
}}

% Python environment
\lstnewenvironment{python}[1][]
{
\pythonstyle
\lstset{#1}
}
{}

% Python for inline
\newcommand\pythoninline[1]{{\pythonstyle\lstinline!#1!}}

\title{Appendix for: ``\crypten{}: Secure Multi-Party Computation Meets Machine Learning''}

% The \author macro works with any number of authors. There are two commands
% used to separate the names and addresses of multiple authors: \And and \AND.
%
% Using \And between authors leaves it to LaTeX to determine where to break the
% lines. Using \AND forces a line break at that point. So, if LaTeX puts 3 of 4
% authors names on the first line, and the last on the second line, try using
% \AND instead of \And before the third author name.

\author{
  Brian Knott
  \quad\quad\quad\enskip Shobha Venkataraman
  \quad\quad\quad\enskip Awni Hannun\\
  \quad\quad\quad\enskip \bf Shubho Sengupta
  \quad\quad\quad\enskip \bf Mark Ibrahim
  \quad\quad\quad\enskip \bf Laurens van der Maaten\\
  Facebook AI Research\\
  \texttt{\{brianknott,shobha,awni,ssengupta,marksibrahim,lvdmaaten\}@fb.com} \\
}

\begin{document}

\maketitle

\appendix
\input{protocols}
\newpage
\input{function_overview}

\newpage
\bibliographystyle{abbrvnat}
\bibliography{references}

\end{document}
